# Supplementary material for: Dr.Occ: Depth- and Region-Guided 3D Occupancy from Surround-View Cameras for Autonomous Driving
Source: arXiv:2603.01007 source file (2026-03-05)
Supplement: Supplementary file 1 [file X_suppl.tex]

\clearpage
\setcounter{page}{1}
\maketitlesupplementary

%这里最好加一个对附件的总体描述，包含哪几部分，每部分讲了啥。

\section{Implementation Details}
\label{sec:implement_details}

\subsection{Deformable Cross-Attention Module Architecture}
\label{sec:supp_dca}
We provide comprehensive architectural specifications of the Deformable Cross-Attention (DCA) module, which serves as the core building block of D$^2$-VFormer. As illustrated in \cref{fig:add-depth}, each DCA module employs a two-stage design: (1) a transformer block for geometric-aware feature learning, and (2) a feature deepening module for progressive refinement.

\noindent\textbf{Transformer Block.} Given input voxel features $\mathbf{F}_{in} \in \mathbb{R}^{N \times C}$, we first apply self-attention to model intra-voxel dependencies. Following standard practice, residual connection and layer normalization stabilize training:
\begin{equation}
\mathbf{F}_{self} = \text{LayerNorm}(\mathbf{F}_{in} + \text{SelfAttn}(\mathbf{F}_{in})).
\end{equation}
Subsequently, we establish geometric correspondence between 3D voxel space and 2D image space through deformable cross-attention, where the normalized features $\mathbf{F}_{self}$ query corresponding image features $\mathbf{F}_{img}$:
\begin{equation}
\mathbf{F}_{cross} = \text{DeformCrossAttn}(\mathbf{Q}=\mathbf{F}_{self}, \mathbf{K},\mathbf{V}=\mathbf{F}_{img}).
\end{equation}
Finally, an FFN with a residual connection further refines the attended features:
\begin{equation}
\mathbf{F}_{trans} = \text{LayerNorm}(\mathbf{F}_{cross} + \text{FFN}(\mathbf{F}_{cross})).
\end{equation}

\noindent\textbf{Feature Deepening Module.} To preserve low-level geometric cues while incorporating high-level semantic information from the transformer, we concatenate the original input $\mathbf{F}_{in}$ with the transformer output $\mathbf{F}_{trans}$:
\begin{equation}
\mathbf{F}_{cat} = [\mathbf{F}_{in}, \mathbf{F}_{trans}] \in \mathbb{R}^{N \times 2C},
\end{equation}
where $[\cdot, \cdot]$ denotes channel-wise concatenation. 
The concatenated features are then processed through a progressive refinement pathway consisting of three 3D convolutional layers ($3 \times 3 \times 3$ kernel) with batch normalization and ReLU activation:
\begin{equation}
\scalebox{0.85}{$\displaystyle
\mathbf{F}_{out} = \text{Conv}_{3}^{C} \circ \text{ReLU} \circ \text{BN} \circ \text{Conv}_{2}^{2C} \circ \text{ReLU} \circ \text{BN} \circ \text{Conv}_{1}^{2C}(\mathbf{F}_{cat}),
$}
\end{equation}
where superscripts denote output channel dimensions. The first two convolutions maintain the expanded dimensionality ($2C$) for sufficient representational capacity, while the final convolution projects back to $C$ dimensions to enable residual connection with subsequent layers. This bottleneck-like design balances feature expressiveness and computational efficiency.
\begin{figure}[t]
    \centering
    \includegraphics[width=0.95\linewidth]{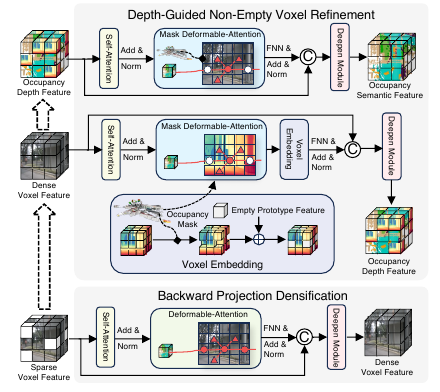}
    \caption{\textbf{Depth-guided Dual Projection View Transformer.}}
    \label{fig:add-depth}
\end{figure}

\subsection{Loss Functions}
\label{sec:supp_loss}
During training, we employ a combination of loss functions to supervise both semantic and geometric learning:
\begin{equation}
    \mathcal{L} = \lambda_{\text{seg}}\mathcal{L}_{\text{seg}} + \lambda_{\text{depth}}\mathcal{L}_{\text{depth}} + \lambda_{\text{sem}}\mathcal{L}_{\text{sem}} + \lambda_{\text{geo}}\mathcal{L}_{\text{geo}},
\end{equation}
where $\mathcal{L}_{\text{seg}}$ denotes the semantic supervision loss with two variants: 
Weight-CELoss employs manually-predefined voxel-level spatial weights that decrease with distance from the ego vehicle. Specifically, for a voxel at position $\mathbf{v} = (x, y, z)$, the weight is defined as $w(\mathbf{v}) = \exp(-\alpha \cdot d(\mathbf{v}))$, where $d(\mathbf{v}) = \sqrt{x^2 + y^2}$ is the distance from the ego vehicle and $\alpha=0.01$ is a decay factor. 
Probability-CELoss adaptively generates voxel-level weights from the model itself. Following ~\cite{i2dlocx, unicalib}, we introduce an auxiliary decoder that estimates the contribution of each voxel by predicting a confidence score $p(\mathbf{v}) \in [0, 1]$. This decoder shares the same feature backbone but outputs a single-channel probability map. The adaptive weight for each voxel is then computed as $w(\mathbf{v}) = p(\mathbf{v})$, enabling the model to automatically learn spatially-varying importance without manual tuning.
In practice, Weight-CELoss is adopted when using the R‑EFormer module, where fixed spatial priors better align with its manually defined regional structure, while Probability-CELoss is employed for the R$^2$‑EFormer variant to leverage its adaptive recursive refinement and dynamically learn voxel-wise importance.
$\mathcal{L}_{\text{depth}}$ follows BEVDepth~\cite{li2023bevdepth} to supervise the forward-projected depth distribution. Following MonoScene~\cite{cao2022monoscene}, we introduce semantic affinity loss $\mathcal{L}_{\text{sem}}$ and geometric affinity loss $\mathcal{L}_{\text{geo}}$ to strengthen supervision on semantic and geometric features. The hyper-parameters are set to $\lambda_{\text{seg}}=10$, $\lambda_{\text{depth}}=1$, $\lambda_{\text{sem}}=1$, and $\lambda_{\text{geo}}=1$, following \cite{cao2022monoscene, flashocc} to maintain consistent optimization scales across losses.

\section{Further Experiments}
\label{sec:supp_ablation}

\subsection{Alternative Depth Integration Strategies}
\label{sec:supp_depth_ablation}
To systematically validate our depth-guided dual projection mechanism, we design comprehensive ablation studies against three representative depth integration strategies (see Table~\ref{tab:supp_depth_strategies} and \cref{fig:lidar_style_comparison}). First, \textit{Direct Depth Replacement} (following BEVDepth~\cite{li2023bevdepth}) substitutes learned depth with externally predicted one-hot depth distributions from MoGe-2~\cite{wang2025moge2}, which causes severe feature–geometry misalignment and leads to a notable drop in occupancy accuracy. Second, \textit{RGBD Concatenation} fuses depth and RGB as a four-channel input using the depth-aware DFormer-v2~\cite{yin2025dformerv2} backbone; although this partially alleviates misalignment, dense depth signals tend to amplify local estimation errors in texture-less or reflective regions, thereby contaminating high-level semantics. Third, \textit{Pseudo-LiDAR Projection} voxelizes depth for LiDAR-style occupancy prediction, as illustrated in \cref{fig:lidar_style_comparison}; this approach suffers from visibility–occupancy gaps, resulting in missing occluded structures and over-densification of visible surfaces. Overall, these comparisons indicate that naive depth injection or direct voxelization disrupts coherent feature learning, whereas our geometry-aware dual projection leverages depth voxels as adaptive geometric priors, achieving superior geometric alignment and semantic consistency.

% \noindent\textbf{Our Depth-Guided Dual Projection.} In sharp contrast, Dr.Occ achieves \textbf{43.43\% mIoU} and \textbf{72.87\% IoU}, surpassing the baseline by \textbf{+7.42\% mIoU} and \textbf{+2.51\% IoU}. 
% This improvement stems from two core designs: 
% (1) a \textit{geometry-aware sparse prior} that explicitly leverages reliable depth cues to identify and emphasize non-empty regions in the voxel space, effectively guiding geometric reasoning in structurally meaningful areas; and 
% (2) a \textit{dual-projection fusion} strategy that decouples geometric alignment from semantic aggregation, allowing feature learning to be adaptively informed by depth rather than constrained by it. 
% These results validate that treating depth as an adaptive geometric prior, instead of a direct input modality, leads to more robust and spatially consistent 3D representations.

\begin{figure}[t]
    \centering
    \includegraphics[width=\linewidth]{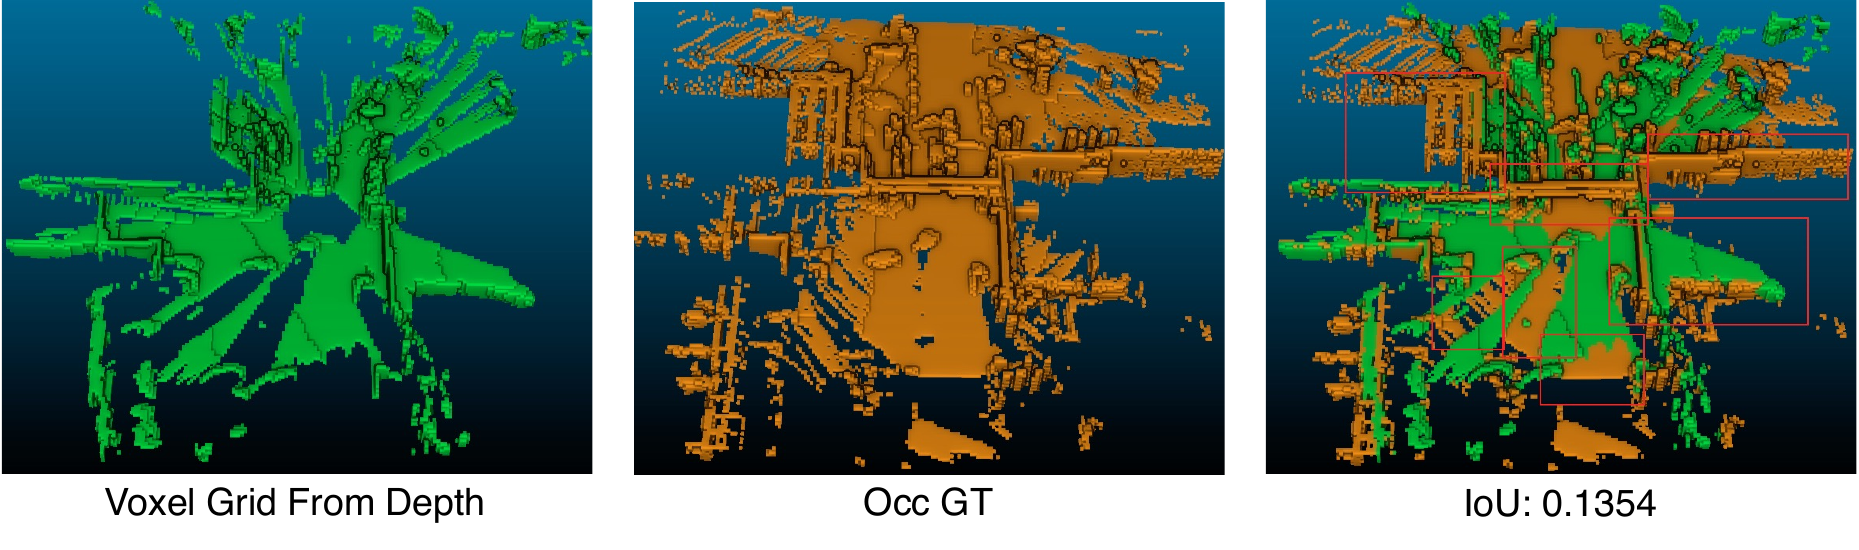}
    \caption{\textbf{Visibility-occupancy mismatch in pseudo-LiDAR projection.} \textbf{Left}: Voxel grid reconstructed from monocular depth. \textbf{Middle}: Occupancy ground truth. \textbf{Right}: Overlay visualization achieving only 13.54\% IoU. Key discrepancies: (1) \textbf{Over-densification}---depth produces dense voxels on visible surfaces where GT is sparse, and (2) \textbf{Occlusion incompleteness}---depth misses occluded regions that GT captures through multi-view aggregation. This fundamental visibility-occupancy gap renders direct depth-to-voxel conversion inadequate for camera-only occupancy prediction.}
    \label{fig:lidar_style_comparison}
\end{figure}

\begin{figure*}[t]
    \centering
    \includegraphics[width=0.78\linewidth]{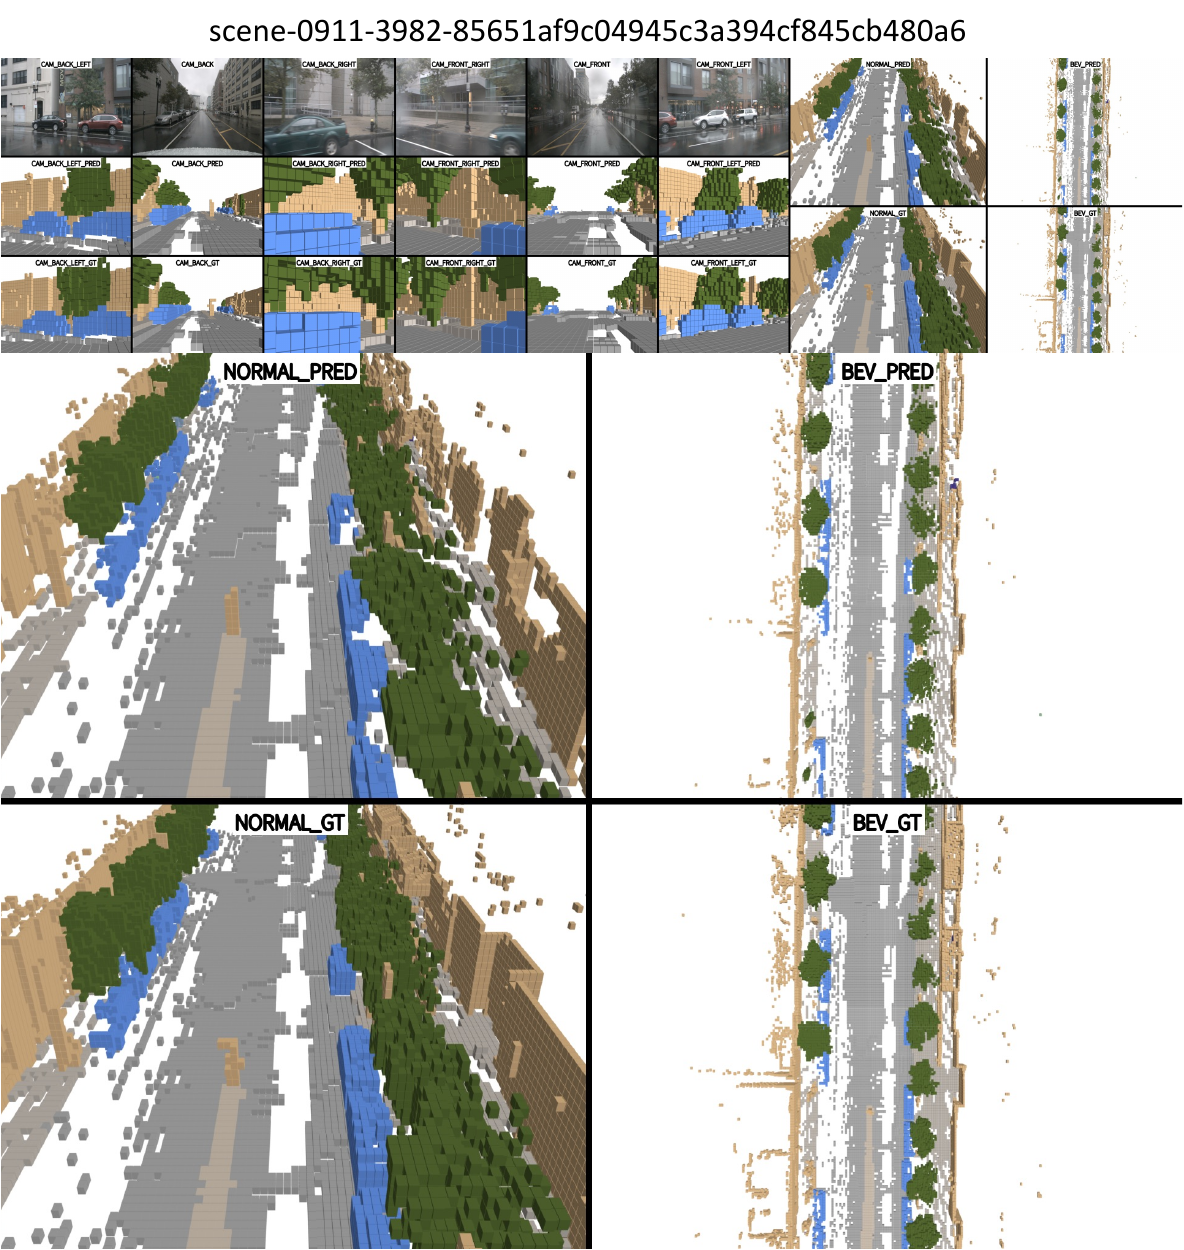}
    \caption{\textbf{Typical case.} Qualitative results show that Dr.Occ recovers road markings, vehicles, buildings, and vegetation with high fidelity, closely matching the ground truth. 
    Readers are encouraged to zoom in to inspect fine-grained geometric and semantic details.}
    \vspace{-3mm}
    \label{fig:vis_normal}
\end{figure*}
\begin{figure*}[t]
    \centering
    \includegraphics[width=0.78\linewidth]{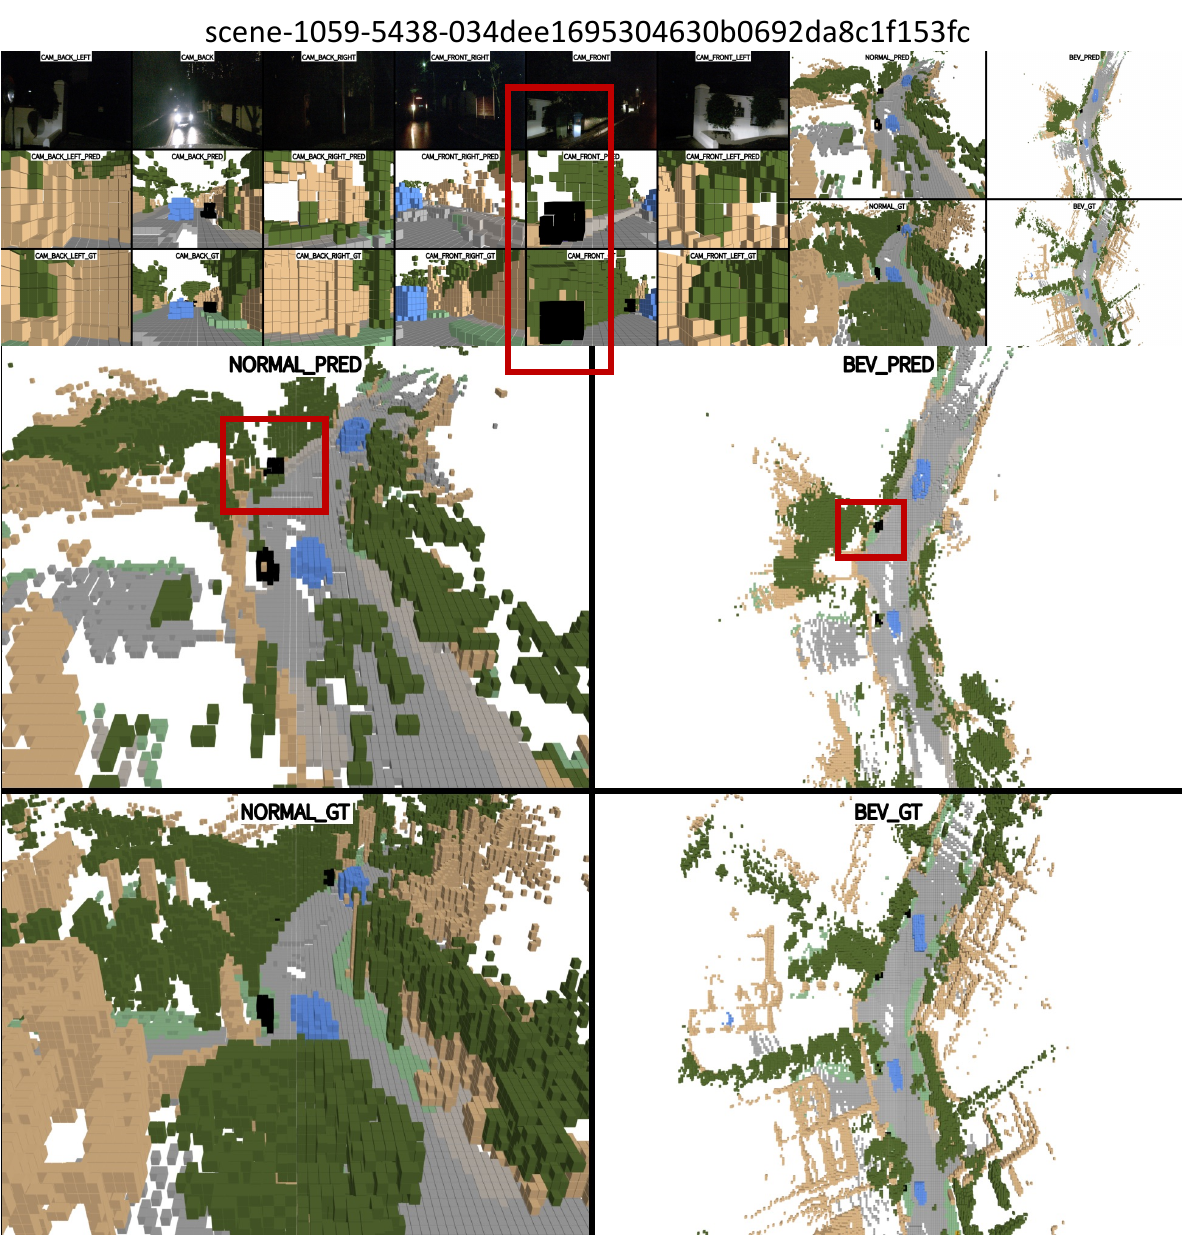}
    \caption{\textbf{Low‑light failure case.} An extremely challenging nighttime scene in which the red box highlights the rare ``others’’ class.  Dr.Occ maintains reasonable predictions despite the severe illumination drop.}
    \vspace{-3mm}
    \label{fig:night_others}
\end{figure*}
\begin{figure*}[t]
    \centering
    \includegraphics[width=0.78\linewidth]{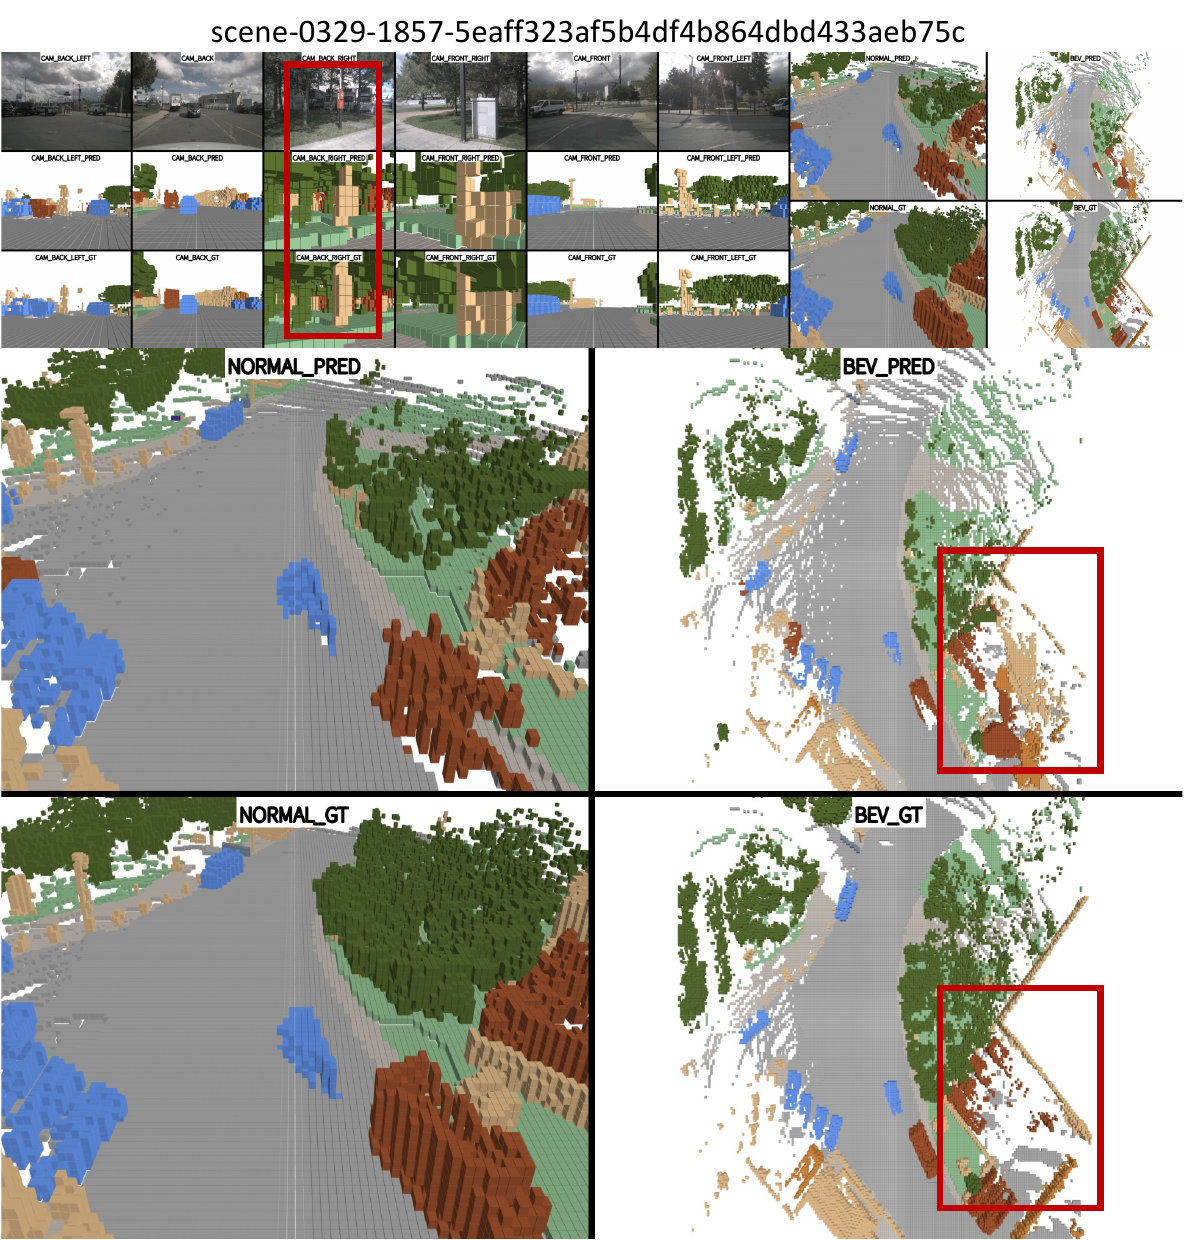}
    \caption{\textbf{Occlusion failure case.} A scene heavily blocked by trees; the model fills in sparse voxels for the visible parts but cannot recover the geometry hidden behind the foliage.}
    \vspace{-3mm}
    \label{fig:tree_occlusion}
\end{figure*}

\begin{table}[t]
  \small
  \centering
  \begin{tabular}{l | c | c c}
      \toprule
      Method & FP Depth & mIoU($\%$) & IoU($\%$) \\
      \midrule
      BEVDet4D (Baseline) & DepthNet & 36.01 & 70.36 \\
      % \hline
      BEVDet4D & MoGe & 18.69 & 60.00 \\
      RGBD-based & DepthNet & 22.97 & 43.49 \\
      % \hline
      Dr.Occ (Ours) & DepthNet & 43.43 & 72.87 \\
  \bottomrule
  \end{tabular}
  \caption{\textbf{Comparison of alternative depth integration strategies on Occ3D-nuScenes.} All methods are built upon BEVDet4D with R50 backbone and 704$\times$256 input resolution. FP Depth denotes the depth source used in forward projection.}
  \label{tab:supp_depth_strategies}
\end{table}

\subsection{Component Analysis of D$^2$-VFormer}
\label{sec:supp_d2vformer_ablation}
\begin{table}[t]
  \small
  \centering
  \begin{tabular}{ccc | c c}
      \toprule
      BP & GR & SE & mIoU($\%$) & IoU($\%$) \\
      \midrule
      & & & 36.01 & 70.36 \\
      \checkmark & & & 39.08 & 70.52 \\
      \checkmark & \checkmark & & 41.16 & 71.07 \\
      \checkmark & \checkmark & \checkmark & 41.45 & 71.29 \\
      \bottomrule
  \end{tabular}
  \caption{\textbf{Ablation study on D$^2$-VFormer components.} BP: Backward Projection Densification; GR: depth-guided Geometric Refinement; SE: depth-guided Semantic Enhancement.}
  \label{tab:supp_d2vformer_ablation}
\end{table}

We conduct comprehensive ablation studies on the three key components of D$^2$-VFormer in Table~\ref{tab:supp_d2vformer_ablation}.
The results demonstrate that each component contributes progressively to performance improvement. Backward Projection Densification (BP) alone brings a substantial gain of +3.07\% mIoU and +0.16\% IoU, validating the effectiveness of dual projection. Adding depth-guided Geometric Refinement (GR) further improves performance by +2.08\% mIoU and +0.55\% IoU, showing that explicit geometric guidance enhances both semantic accuracy and occupancy prediction. Finally, incorporating Semantic Enhancement (SE) yields additional improvements of +0.29\% mIoU and +0.22\% IoU. The cumulative gains demonstrate that all three components effectively contribute to our final design, achieving +5.44\% mIoU and +0.93\% IoU over the baseline.

\subsection{Runtime Analysis}
\label{sec:supp_efficiency}
As reported in Table~\ref{tab:runtime_compo}, we analyze the runtime characteristics of each component in our framework. 
The \textbf{baseline (BL)} configuration represents the standard feature extraction and projection pipeline, while \textbf{Depth Cues (DC)} serve as the default geometric prior provided by MoGe‑2~\cite{wang2025moge2}. DC introduces only a minor runtime overhead of 37\,ms, making it an efficient default setting for all subsequent modules.
The \textbf{D$^2$‑VFormer (D2V)} requires 144\,ms due to dual‑projection and depth‑guided deformable fusion, reflecting a deliberate trade‑off that substantially improves 3D geometric alignment and voxel representation quality. 
The \textbf{R‑EFormer (RE)} exhibits the highest runtime (313\,ms) as its multi‑expert routing performs region‑wise semantic reasoning across the entire volume, leading to significant accuracy gains but a large computational burden. 
To address this limitation, the recursive variant \textbf{R$^2$‑EFormer (R2E)} replaces multiple experts with a single recursively applied one, reducing runtime to 72\,ms while preserving the semantic discrimination. 
This analysis highlights that although modules such as D2V and RE are computationally demanding, each substantially contributes to representation quality, and the recursive refinement in R2E achieves an effective balance between accuracy and efficiency. 

Although our latency (337ms vs. 84ms) and memory usage (5.5GB vs. 2.9GB) increase, these costs remain well within the operational envelope of modern automotive SoCs (e.g., NVIDIA Orin). The substantial +7.4\% mIoU gain
represents a significant leap in perception quality that sim- ple scaling the baseline cannot achieve, as efficiency-centric models often hit a performance ceiling due to geometric loss. Our model is also practical to train, requiring 38GB VRAM per GPU (BS=2). Finally, the proposed decoupled design allows heavy attention components to be replaced with hardware-friendly operators for reduced latency. 

\begin{table}[t]
\centering
\resizebox{\linewidth}{!}{
\begin{tabular}{lccccc}
    \toprule
     & \textbf{BL} & \textbf{DC} & \textbf{D2V} & \textbf{RE} & \textbf{R2E} \\ 
    \midrule
    \textbf{Time [ms]} & 84 & 37 & 144 & 313 & 72  \\
    \bottomrule
\end{tabular}
}
\caption{\textbf{Runtime Performance of Each Component.}
BL: Baseline; DC: Depth Cues; D2V: D$^2$‑VFormer; RE: R‑EFormer; R2E: R$^2$‑EFormer.}
\vspace{-5mm}
\label{tab:runtime_compo}
\end{table}

\section{Additional Qualitative Results}
\label{sec:supp_qualitative}
In this section, we provide qualitative visualizations to illustrate the prediction quality and robustness of Dr.Occ. The first example shows a typical scene to familiarize the reader with our visualization layout, while the latter two examples highlight challenging conditions, including low-light and heavy occlusion (see Fig.~\ref{fig:vis_normal}, Fig.~\ref{fig:night_others}, and Fig.~\ref{fig:tree_occlusion}).

\paragraph{Typical Scene.}
Figure~\ref{fig:vis_normal} presents a representative daytime scene. The top three rows show the six synchronized RGB camera views, the predicted occupancy (\texttt{Occ pred}), and the ground-truth occupancy (\texttt{Occ GT}). On the right, we visualize the scene in a BEV view and a 3D top-down perspective view, with enlarged crops displayed below for clarity. These visualizations demonstrate that Dr.Occ can produce occupancy maps that align well with the ground truth and capture fine-grained geometric and semantic details across multiple perspectives.

\paragraph{Low-light Scenes.}
We then examine an extremely challenging nighttime example (scene–1059, Fig.~\ref{fig:night_others}). Specifically, the red bounding box denotes the rare ``others’’ category; despite the severely degraded illumination, Dr.Occ successfully detects this low-frequency class and generates a reasonable occupancy map. However, in completely dark image regions, the network tends to predict empty space, suggesting that additional sensing modalities (e.g., LiDAR or radar) are needed to recover missing occupancy information.

\paragraph{Occluded Scenes.}
Finally, we probe the limits of the framework under significant vegetation occlusion (scene–0329, Fig.~\ref{fig:tree_occlusion}). Dr.Occ reconstructs sparse voxels corresponding to the visible portions of the scene, but the details hidden behind the canopy remain unrecoverable due to the lack of visual cues. As with the low-light failure case, complete recovery would require complementary sensors such as LiDAR or radar.

\paragraph{Summary.}
Together with the results presented in the main paper, these visualizations confirm that Dr.Occ can generate reliable occupancy predictions in both typical and adverse conditions, while also making its current limitations explicit. Future work will explore multimodal fusion to address these failure scenarios.
