# Supplementary material for: Dr.Occ: Depth- and Region-Guided 3D Occupancy from Surround-View Cameras for Autonomous Driving
Source: arXiv:2603.01007 source file (2026-03-05)
Supplement: Supplementary file 2 [file additional_ab.tex]

\begin{table}[t]
  \small
  \centering
  \begin{tabular}{ccc | c c}
      \toprule
      BP & GR & SE & mIoU($\%$) & IoU($\%$) \\
      \midrule
      & & & 36.01 & 70.36 \\
      \checkmark & & & 39.08 & 70.52 \\
      \checkmark & \checkmark & & 41.16 & 71.07 \\
      \checkmark & \checkmark & \checkmark & 41.45 & 71.29 \\
      \bottomrule
  \end{tabular}
  \caption{\textbf{Ablation study on D$^2$-VFormer components.} BP: Backward Projection Densification; GR: depth-guided Geometric Refinement; SE: depth-guided Semantic Enhancement.}
  \label{tab:supp_d2vformer_ablation}
\end{table}
